# Supplementary material for: Secure Computation over Encrypted Databases
Source: arXiv:2308.02878 source file (2023-08-05)
Supplement: Supplementary file 1 [file appendix.tex]

\newpage
\section{Appendix}

In this section we will present a toy example which will be handy to understand the proposed encryption scheme. Let the DO have database $\boldsymbol{\mathcal{D}} = (\boldsymbol{p}_1,\boldsymbol{p}_2)$ with $d=2$ as $\boldsymbol{p}_1=(6,7)$ and $\boldsymbol{p}_2=(4,5)$. For encryption DO samples security parameters $\epsilon=4$ and $c=2$ as security parameters, evaluating $\eta$ to $\eta=d+2+c+\epsilon=10$.

\textbf{KeyGen:}: In this step of the encryption scheme secret matrix and different secret vectors are sampled as follows: \\ 

\begin{align*}
\mathbf{M} &=\begin{bmatrix}
8.5  &  3.2  &  4.3  &  1.8  &  2.1  &  3.5  &  5.9  &  8.6  &  7.2  &  1.3 \\
1.6  &  4.7  &  3.1  &  2.9  &  6.3  &  9.1  &  3.8  &  4.1  &  2.3  &  2.9 \\
2.1  &  7.2  &  8.5  &  1.9  &  2.5  &  8.9  &  9.1  &  5.1  &  7.1  &  9.8 \\
2.3  &  4.9  &  1.1  &  5.6  &  4.2  &  1.8  &  2.6  &  5.5  &  2.7  &  7.3 \\
5.1  &  3.4  &  7.2  &  3.7  &  8.3  &  1.5  &  6.9  &  7.5  &  9.2  &  6.6 \\
9.5  &  3.5  &  1.1  &  8.3  &  6.3  &  1.8  &  2.9  &  6.1  &  5.6  &  7.8 \\
7.9  &  9.4  &  7.8  &  5.6  &  3.2  &  4.8  &  2.3  &  3.8  &  3.2  &  9.4 \\
5.7  &  6.4  &  6.9  &  2.8  &  7.9  &  9.6  &  4.6  &  5.1  &  1.4  &  8.3 \\
1.8  &  5.8  &  1.4  &  4.1  &  3.8  &  4.7  &  7.1  &  4.4  &  3.8  &  5.9 \\
8.4  &  3.4  &  7.3  &  2.9  &  5.5  &  6.7  &  6.1  &  6.7  &  7.2  &  3.3 \\
\end{bmatrix}\\
\boldsymbol{s} &=(15,63,17) \\
% The $d$-dimensional long term secret vector
\boldsymbol{\sigma} &=(8,11) \\
% $(c+\epsilon)$-dimensional bit string 
\boldsymbol{b} &=(1,1,1,0,1,0) \\
% The $(c+\epsilon)$-dimensional weight point 
\boldsymbol{w} &=(19,23,11,18,25,40) \\
% The permutation function 
\boldsymbol{\pi} &=(5,2,7,1,8,4,3,6,0,9)
\end{align*}

The secret key of DO have components: $(\boldsymbol{\mathbf{M}},\boldsymbol{s},\boldsymbol{\sigma},\boldsymbol{b},\boldsymbol{w},\boldsymbol{\pi})$

\textbf{Tuple Encryption:}: In this step of the encryption scheme data point encryption is performed using the secret key as mentioned above. For encrypting $\boldsymbol{p}_1=(6,7)$, DO computes the $(c+\epsilon)=6$-dimensional per data point ephemeral secret  $\boldsymbol{\tau}_1$ using $\boldsymbol{b}$ and $\boldsymbol{w}$ as \begin{align*}
\tau_{10} &=w_1   =19 \ \ as \ b_1 = 1 \\
\tau_{11} &=w_2   =23 \ \ as \ b_2 = 1 \\
\tau_{12} &=w_3   =11 \ \ as \ b_3 = 1 \\
\tau_{13} &=rand  =3 \ \ as \ b_4 = 0 \\
\tau_{14} &=w_4   =25 \ \ as \ b_5 = 1 \\
\tau_{15} &=-nom_p =-42.25 \ \ as \ b_6 =0\ (last\ 0) \\
\end{align*}
For computing $nom_p$ following computation is performed
\begin{align*}
\boldsymbol{\tau}_{1}\boldsymbol{w} &=0\\
19*19+23*23+11*11+ & 18*3+25*25+40*nom_p =0 \\
nom_p &= -42.25
\end{align*}

Then computes $\alpha_1$ as
$$\alpha_1=(\sigma_1-t_1)^2 + (\sigma_2-t_2)^2=(8-7)^2+(11-4)^2=50 $$
with randomly sampled $(t_1,t_2)=(7,4)$

Now, DO creates $\hat{\boldsymbol{p}}_1$ as 
\begin{align*}
& (s_1-2p_{11},s_2-2p_{12},\cdots,s_d-2p_{1d}, s_{d+1}+\Vert \boldsymbol{p}_1 \Vert^{2}, \alpha_1, \boldsymbol{\tau}_1) \\
&= (3, 49, 102, 50, 19, 23, 11, 3, 25, -42.25)   
\end{align*}

Then encrypts it by computing 
\begin{align*}
\boldsymbol{p}_1' &= \hat{\boldsymbol{p}}_1\mathbf{\hat{M}^{-1}} \\
&= (-2.450,4.596,-20.674,-4.666,1.680,-14.833,\\ & 16.390,-10.106,30.685,11.411)
\end{align*}

Similarly, second data point is encrypted to obtain the encrypted data point as 
\begin{align*}
\boldsymbol{p}_2' &=
(-21.880,-19.894,-24.697,15.103,-9.657,\\
& -24.043,4.931,-7.558,44.538,54.709)
\end{align*}

\textbf{Query Encryption:}: Let the QU have query point $\boldsymbol{q}_2=(3,9)$ and he wants to figure out the $1$-NN. Thus he samples $(sk,pk)$ of Paillier encryption scheme and encrypts the query point $\boldsymbol{q}$ to obtain $\dot{\boldsymbol{q}} = (E_{pk}(3), E_{pk}(9))$ and sends the $(\dot{\boldsymbol{q}},pk)$ to the DO. DO samples a random number $\beta_1=4$ and computes  $\beta_2=44$. 

QU performs the random permutation of $\{0,1\}$ to obtain a permutation vector $v=(0,1)$ and computes $\frac{d}{c}=1$. Then computes $\boldsymbol{r}^{enc}$, a $(c+\epsilon)$-dimensional point as
\begin{align*}
r^{enc}_0 &= -E_{pk}(3)^{2100}   =-E_{pk}(6300) \ as \  j=0  \ and\ b_0=1  \\
r^{enc}_1 &= -E_{pk}(9)^{200}    =-E_{pk}(1800) \ as \  j=1  \ and\ b_1=1  \\
r^{enc}_2 &= -E_{pk}(rand)^{100} =-E_{pk}(600)  \ as \  b_2=1   \\
r^{enc}_3 &= -E_{pk}(w_3)^{100}  =-E_{pk}(1800) \ as \  b_3=0   \\
r^{enc}_4 &= nom_q               =E_{pk}(14404)   \ as \  b_4=1\ (last \ 1)   \\
r^{enc}_5 &= -E_{pk}(w_5)^{100}  =-E_{pk}(4000) \ as \  b_5=0   \\
\end{align*}

Here each element is multiplied with $100$ so that $nom_q$ will be an integer. Here $nom_q$ is computed as shown by equation \ref{nom_q_calculation}.

\begin{align}
\boldsymbol{r}^{enc}\boldsymbol{w} &=E_{pk}(0)\nonumber \\    
(r^{enc}_0)^{w_0}*(r^{enc}_1)^{w_1}*\cdots*(r^{enc}_5)^{w_5} &= E_{pk}(0)\nonumber \\
E_{pk}(6300*19+ \cdots +40*4000) &= E_{pk}(25*nom_q)\nonumber\\
E_{pk}(nom_q)^{25} &=E_{pk}(360100)\nonumber\\
E_{pk}(nom_q) &=E_{pk}(14404)
\label{nom_q_calculation}
\end{align}

% \begin{figure*}[!t]
% % ensure that we have normalsize text
% \normalsize
% % Store the current equation number.

% % \setcounter{MYtempeqncnt}{\value{equation}}

% % Set the equation number to one less than the one
% % desired for the first equation here.
% % The value here will have to changed if equations
% % are added or removed prior to the place these
% % equations are referenced in the main text.
% \hrulefill
% \begin{align*}
% \boldsymbol{r}^{enc}\boldsymbol{w} &=E_{pk}(0)\\    
% (r^{enc}_0)^{w_0}*(r^{enc}_1)^{w_1}*(r^{enc}_2)^{w_2}*(r^{enc}_3)^{w_3}* & (r^{enc}_4)^{nom_q}*(r^{enc}_5)^{w_5} = E_{pk}(0) \\
% E_{pk}(25*nom_q) = E_{pk}(6300*19+&1800*23+600*11+1800*18 +40*4000) \\
% E_{pk}(nom_q)^{25} &=E_{pk}(360100)\\
% E_{pk}(nom_q) &=E_{pk}(14404)
% \end{align*}

% \hrulefill
% % The spacer can be tweaked to stop underfull vboxes.
% % \vspace*{4pt}
% \label{Claim}
% \caption{Computation of $nom_q$ value}
% \end{figure*}

Now, compute $\overline{\boldsymbol{q}}$ as
\begin{align*}
\overline{\boldsymbol{q}} &=(\dot{q}_{1}^{\beta_2},\dot{q}_{2}^{\beta_2},E_{pk}(\beta_2), E_{pk}(\beta_1), \boldsymbol{r}^{enc}) \\
&=\pi(E_{pk}(13200), E_{pk}(39600), E_{pk}(4400), E_{pk}(400), -E_{pk}(6300),\\  & -E_{pk}(1800), -E_{pk}(600), -E_{pk}(1800), E_{pk}(14404), -E_{pk}(4000))\\
&=(-E_{pk}(1800), E_{pk}(4400), -E_{pk}(1800), E_{pk}(39600), E_{pk}(14404),\\  & -E_{pk}(6300), E_{pk}(400), -E_{pk}(600), E_{pk}(13200), -E_{pk}(4000))
\end{align*}

Finally, ciphertext $\mathbf{{a}}^{(q)}$ is computed as 
\begin{align*}
\mathbf{{a}}^{(q)} &= (a_1^{(q)},a_2^{(q)},\cdots,a_{\eta}^{(q)}) \\
&= (\prod_{j=1}^{\eta}  \overline{\boldsymbol{q}}_j^{\boldsymbol{\hat{M}}_{1,j}}, \prod_{j=1}^{\eta}  \overline{\boldsymbol{q}}_j^{\boldsymbol{\hat{M}}_{2,j}},\cdots, \prod_{j=1}^{\eta}  \overline{\boldsymbol{q}}_j^{\boldsymbol{\hat{M}}_{\eta,j}}) \\
&= (E_{pk}(1575584), E_{pk}(1782952), E_{pk}(1228800), E_{pk}(2905368), \\ & E_{pk}(3427432), E_{pk}(4446252), E_{pk}(2539928), E_{pk}(1537316),\\& E_{pk}(2340052), E_{pk}(2188120))
\end{align*}

Here secret matrix $\boldsymbol{\hat{M}}$ is multiplied with $10$ to convert its elements into integers then multiplied with $\overline{\boldsymbol{q}}$ to obtain the final ciphertext $\mathbf{{a}}^{(q)}$.

Received encrypted ciphertext $\mathbf{{a}}^{(q)}$ is decrypted by QU to obtain $\boldsymbol{q}'$ as
\begin{align*}
\boldsymbol{q}' &= D_{sk}(\mathbf{{a}}^{(q)})\\
     &= (1575584, 1782952, 1228800, 2905368, 3427432, 4446252,\\& 2539928, 1537316, 2340052, 2188120)
\end{align*}
$\boldsymbol{q}'$ is then send to CSP for $k$-NN computation.  
\newpage
\textbf{Secure $k$-NN Computation:} In this step CSP performs multiplication of data points with query point. To obtain values as 
\begin{align*}
    \boldsymbol{p}_1'\boldsymbol{q}' &= 28048002.560 \\ 
    \boldsymbol{p}_2'\boldsymbol{q}' &= 28424001.890
\end{align*}                       

Thus CSP reports the data point index $0$ as $1$-NN to the QU.
The same can be verified by computing $1$-NN in the plaintext domain as 
\begin{align*}
    \boldsymbol{p}_1\boldsymbol{q} &= (6-3)^2+(7-9)^2=13 \\ 
    \boldsymbol{p}_2\boldsymbol{q} &= (4-3)^2+(5-9)^2=17 \\
\end{align*}      
Thus the proposed encryption indeed computes the correct nearest neighbor in the encrypted domain. This completes our toy example.

\newpage

% \begin{table}[!h]
%     \centering
%     \begin{tabular}{|c|c|c|c|c|}
%      \hline
%      \multirow{Encrypted Tuples in Database} & \multicolumn{4}{|c|}{Known Plaintexts} & 
%      \cline{2-5}
%     %  \vspace{.001em}
%      & $\makecell{(\boldsymbol{p}_{i_{1}}) \vspace{.5em} \\  s_1' s_2' \cdots s_d'}$ & $\makecell{(\boldsymbol{p}_{i_{2}}) \vspace{.5em} \\ s_1' s_2' \cdots s_d'}$ & $\cdots$ & $\makecell{(\boldsymbol{p}_{i_{k}}) \vspace{.5em} \\  s_1' s_2' \cdots s_d'}$ \\
%     \cline{2-5}
%     \hline
%     % \vspace{.001em}
%     $\boldsymbol{p}_1'$ & $123 \ 939 \cdots 478$ & $571 \ 286 \cdots 329$ & $\cdots$ & $295 \ 310 \cdots 836$ \\
%     \hline
%     % \vspace{.001em}
%     $\boldsymbol{p}_2'$ & $752 \ 083 \cdots 906$ & $472 \ 388 \cdots 512$ & $ \ \ \ \ \ \ \ \ \cdots \ \ \ \ \ \ \ \ $ & $185 \ 364 \cdots 280$ \\
%     \hline
    
%     $\vdots$ & $\vdots$ & $\vdots$ & $\vdots$ & $\vdots$ \\
%     \hline
%     % \vspace{.001em}
%     $\boldsymbol{p}_t'$ & $295 \ 310 \cdots 836$ & $065 \ 387 \cdots 926$ & $\cdots$ & $693 \ 377 \cdots 598$\\
    
%     \hline
%     \end{tabular}
%     \vspace{1em}
%      \caption{Table aiding the attack technique} 
%      \vspace{-.5cm}
%      \label{Attack_Tab}
% \end{table}
